# Supplementary material for: Fluid Control with Localized Spacetime Windows
Source: arXiv:2511.15189 source file (2026-06-18)
Supplement: Supplementary file 1 [file supplemental.tex]

\section{Appendix}
\label{sec:appendix}
